# Supplementary material for: S2HPruner: Soft-to-Hard Distillation Bridges the Discretization Gap in Pruning
Source: arXiv:2410.07046 source file (2024-10-09)
Supplement: Supplementary file 1 [file appendix.tex]

\setcounter{section}{0}
\setcounter{figure}{6}
\setcounter{table}{6}
\setcounter{equation}{4}

\iffalse
4 videos
    4 ablation study?
    5 more 
    1 comparison of text-to-motion
    2 comparison of action-to-motion
    3 comparison of uncondition
    
1 3.1-the supervision and more implementation details are listed in the
supplements.
2 4-Experiments More qualitative results and user studies are provided in supplements.
\fi

This appendix provides more qualitative results (\cref{sec:appendix:qualitative}), 
several additional experiments (\cref{sec:appendix:exps}) on the components of motion latent diffusion (MLD) models, 
evaluations of inference time (\cref{sec:appendix:inferencetime}),
visualization of latent space (\cref{sec:appendix:tsne}),
evaluations on hyperparameters (\cref{sec:appendix:hyperparameters}), 
user study (\cref{sec:appendix:userstudy}), 
details of motion representations (\cref{sec:appendix:motionRepre}), 
implementation details of MLD models (\cref{appedix:method:detail}) and metric definitions (\cref{appedix:metrics:details}).\\

% \myparagraph{Video.} We have provided the supplemental video to illustrate our results. In this video, we show 1) comparisons of text-based motion generation, 2) comparisons of action-conditional motion generation, and 3) more samples of unconditional generation. We suggest the reader watch this video for dynamic motion results.\\

% \myparagraph{Code} is available in supplements. We provide example code files, which include the process of the training and evaluation of our MLD models, the LOG files of models and evaluations (the model file is too large to upload), and example results.

\myparagraph{Video.} We have provided supplemental videos in \href{https://chenxin.tech/mld}{Project Page}. In these supplemental videos, we show 1) comparisons of text-based motion generation, 2) comparisons of action-conditional motion generation, and 3) more samples of unconditional generation. We suggest the reader watch this video for dynamic motion results.\\

\myparagraph{Code} is available on \href{https://github.com/chenfengye/motion-latent-diffusion}{GitHub Page}. We provide the process of the training and evaluation of MLD models, the pre-trained model files, the demo script, and example results.

\section{Qualitative Results}
\begin{figure}[h]
    \centering
    \includegraphics[width=\linewidth]{figures/comp_action.pdf}
    \caption{The comparison of the state-of-the-art methods on action-conditional motion synthesis task. All provided methods are under the same training and inference setting on HumanAct12 dataset~\cite{guo2020action2motion}. We generate three motions for each action label. The results demonstrate that our generations correspond better to the action label and have richer diversity.}
    \label{fig:appendix:action}
\end{figure}

\label{sec:appendix:qualitative}
\begin{figure}[h]
    \centering
    \includegraphics[width=0.955\linewidth]{figures/more_rs.pdf}
    \caption{More samples from our best model for text-to-motion synthesis, \textit{MLD-1}, which was trained on the HumanML3D dataset. Samples generated with text prompts of the test set. We recommend the supplemental video to see these motion results. }
    \label{fig:appendix:more_rs}
\end{figure}

% 1 Qualitative results.
%   1.1 our more results
  
%   1.2 more comparisons
%         action-comparison
        
  % 1.3 ablation study xx ?

\newpage
\section{Additional Experiments}
\label{sec:appendix:exps}
We conduct several experiments to continue the evaluations of MLD models. We first study the influence of language models $\tau_\theta^w$ and the shape of text embedding on motion generations. Then, we evaluate the effectiveness of long skip connections for motion diffusion models. We finally study the importance of regularization on motion latent space.  
% xxx metrics better than the main scripts xx

% \subsection{Diffusion on Latent or Motion}
% \label{mdm-like}
% mdm-like\cite{mdm2022Autoenchuman}

\subsection{Evaluation of Language Models $\tau_\theta^w$ }
We experiment with different language models, CLIP~\cite{radford2021learning} and BERT~\cite{devlin2018bert}. 
Inspired by Stable Diffusion~\cite{stable_diffusion}, we leverage the hidden state of CLIP to generate word-wise tokens and explore its effects.
The comparisons are listed in \cref{tab:appendix:language}. CLIP is more suited to our task compared to BERT, and the word-wise text tokens are competitive with the single token, however, lower the computation efficiency of diffusion models.
Therefore, we choose CLIP and a single text token for our models.

\begin{table}[h]
\centering
\resizebox{0.8\columnwidth}{!}{%
\begin{tabular}{@{}lccccccc@{}}
\toprule
\multirow{2}{*}{Models} & Text Encoder& Embeddings & \multicolumn{1}{c}{R Precision} & \multicolumn{1}{c}{\multirow{2}{*}{FID$\downarrow$}} &  \multirow{2}{*}{MM Dist$\downarrow$} & \multirow{2}{*}{Diversity$\rightarrow$} & \multirow{2}{*}{MModality$\uparrow$} \\
                          & $\tau_\theta^w$ &Shape & \multicolumn{1}{c}{Top 3$\uparrow$}       & \multicolumn{1}{c}{}                     &                          &                            &     \\ \toprule
% $\tau_\theta^w(w^{1:N})$
Real & - & - &
  $0.797^{\pm.002}$ &
  $0.002^{\pm.000}$ &
  $2.974^{\pm.008}$ &
  $9.503^{\pm.065}$ &
  \multicolumn{1}{c}{-}
  \\ \midrule
MLD-1 & BERT~\cite{devlin2018bert}& $1\times256$ 
&$0.725^{\pm.002}$&	$0.553^{\pm.020}$&	$3.530^{\pm.011}$&	$\boldsymbol{9.697}^{\pm.080}$&	$\boldsymbol{3.360}^{\pm.118}$
%&$0.684^{\pm.003}$ &	$0.646^{\pm.020}$ &	$3.767^{\pm.012}$ &	$\boldsymbol{9.758}^{\pm.081}$ &	$\boldsymbol{3.602}^{\pm.121}$
  \\
MLD-1 & CLIP~\cite{radford2021learning}   & $1\times256$
& $\boldsymbol{0.769}^{\pm.002}$ &	$0.446^{\pm.011}$&	$\boldsymbol{3.227}^{\pm.010}$&	$9.772^{\pm.071}$&	$2.413^{\pm.072}$\\
MLD-1 & CLIP~\cite{radford2021learning} & $77\times256$& $0.737^{\pm.002}$	& $\boldsymbol{0.422}^{\pm.012}$	& $3.436^{\pm.010}$ &	$9.840^{\pm.082}$ &	$2.799^{\pm.107}$   \\

\bottomrule
\end{tabular}%
}
% \vspace{2pt}
\caption{Quantitative comparison of the employed language models. Here we set batch size to 500 and only change the text encoder $\tau_\theta^w$. }
\label{tab:appendix:language}
\end{table}

\subsection{Effectiveness of Long Skip Connection}
We have demonstrated the effectiveness of skip connection, especially on diffusion models in \cref{tab:ablation:diffusion}. Here we analyze its influence on the training of diffusion stage. As shown in \cref{fig:appendix:skip}, the model with long skip connection not only achieves higher performance but also provides faster convergence compared to the other one. The results suggest leveraging long skip connections for iterative motion diffusion models.

\begin{figure}[h]
    \centering
    \includegraphics[width=0.7\linewidth]{figures/appendix_curve.pdf}
    \vspace{-10pt}
    \caption{The evaluation on long skip connection on diffusion training stage. Two sub-figures are under the same training process and evaluated on the test set of HumanML3D. Training steps indicate the epoch number.}
    \label{fig:appendix:skip}
\end{figure}
% 增加收敛效果的对比图

% 也可以单领一个章节 说明 skip connection放在diffusion里可以帮助diffusion网络快速收敛
% 放一个网络收敛的折线波动图
% 参考 - fid
% MDiffuse_1028_VaeMcross_lat5_transenc9_bs500_skip_lr1e4_cliphidden_75_vae15399
% MDiffuse_1028_VaeMcross_lat5_transenc8_bs500_lr1e4_cliphidden_75_vae15399

\subsection{Diffusion on Autoencoder or VAE}
% E. autoencoder v.s. vae for diffusion models
We study the importance of regularization on motion latent space. The regularized latent space provides stronger generation ability and supports the latent diffusion models as demonstrated:

\begin{table}[H]
\centering
\resizebox{0.65\columnwidth}{!}{%
\begin{tabular}{@{}lccccccl@{}}
\toprule
\multirow{2}{*}{Method} & \multicolumn{3}{c}{Reconstruction}                            &  \multicolumn{2}{c}{Generation}        \\ \cmidrule(lr){2-4} \cmidrule(l){5-6} 
                        & MPJPE $\downarrow$ & PAMPJPE$\downarrow$ & ACCL$\downarrow$ &   FID$\downarrow$& DIV$\rightarrow$\\ \midrule
% Real  &  \multicolumn{1}{c}{-} & \multicolumn{1}{c}{-}& \multicolumn{1}{c}{-} &  $0.002\hidden{^{\pm.000}}$&	$9.503\hidden{^{\pm.065}}$     \\ \midrule

Autoencoder & {38.5} &  {28.2} & 5.8 & 0.156 & 9.628
%& 38.5& 28 & 5.8 & 0.156 & 9.628
\\
% 7 256
VAE & $\boldsymbol{14.7}$ & $ \boldsymbol{8.9}$ & $\boldsymbol{5.1}$ & $\boldsymbol{0.017}\hidden{^{\pm.000}}$ &  $\boldsymbol{9.554}\hidden{^{\pm.062}}$
\\ 
\bottomrule
\toprule

\multirow{2}{*}{Method} & \multicolumn{1}{c}{R Precision} & \multicolumn{1}{c}{\multirow{2}{*}{FID$\downarrow$}} & \multirow{2}{*}{MM Dist$\downarrow$} & \multirow{2}{*}{Diversity$\rightarrow$} & \multirow{2}{*}{MModality$\uparrow$} \\
                          & \multicolumn{1}{c}{Top 3$\uparrow$}       & \multicolumn{1}{c}{}                     &                          &                            &     \\ \toprule
% Real &
%   $0.797^{\pm.002}$ &
%   $0.002^{\pm.000}$ &
%   $2.974^{\pm.008}$ &
%   $9.503^{\pm.065}$ &
%   \multicolumn{1}{c}{-}
%   \\ \midrule
MLD w/ Autoencoder & $0.581^{\pm.003}$ &	$5.033^{\pm.061}$ &	$4.600^{\pm.018}$ &	$7.953^{\pm.083}$ &	$\boldsymbol{3.754}^{\pm.111}$
 \\
MLD w/ VAE & 
$\boldsymbol{0.772}^{\pm.002}$ &	$\boldsymbol{0.473}^{\pm.013}$ &	$\boldsymbol{3.196}^{\pm.010}$ &	$\boldsymbol{9.724}^{\pm.082}$ &	$2.413^{\pm.079}$
%$\boldsymbol{0.771}^{\pm.003}$ & $\boldsymbol{0.402}^{\pm.011}$ &	$\boldsymbol{3.203}^{\pm.013}$ &	$\boldsymbol{9.876}^{\pm.088}$ &	$2.478^{\pm.076}$  

\\ \bottomrule
\end{tabular}%
}
% \vspace{2pt}
\caption{Evaluation of autoencoder (without  Kullback-Leibler regularization) and VAE model on motion generations.}
\label{tab:supp:ablation}
\end{table}

\subsection{Prediction of Denoising}
\label{sec:appendix:predictdenoising}

We compare predicting the denoised latent vector $z_0$ directly instead of $\epsilon$ in the denoising process. 
\cref{tab:tm:abl:humanml3d} shows that the latter performs better, which verifies the proposal from DDPM ~\cite{ho2020denoising}.

\begin{table}[h]
% \vspace{-12pt}
\centering
\resizebox{0.8\columnwidth}{!}{%
\begin{tabular}{@{}lccccccc@{}}
\toprule
\multirow{2}{*}{Methods} & \multicolumn{3}{c}{R Precision $\uparrow$}& \multicolumn{1}{c}{\multirow{2}{*}{FID$\downarrow$}} & \multirow{2}{*}{MM Dist$\downarrow$}& \multirow{2}{*}{Diversity$\rightarrow$} & \multirow{2}{*}{MModality$\uparrow$}\\ \cmidrule(lr){2-4} & \multicolumn{1}{c}{Top 1} & \multicolumn{1}{c}{Top 2} & \multicolumn{1}{c}{Top 3} & \multicolumn{1}{c}{} &&&\\ \midrule
% Real &
%   $0.511^{\pm.003}$ &
%   $0.703^{\pm.003}$ &
%   $0.797^{\pm.002}$ &
%   $0.002^{\pm.000}$ &
%   $2.974^{\pm.008}$ &
%   $9.503^{\pm.065}$ &
%   \multicolumn{1}{c}{-}
%   \\ \midrule
MLD-1 ($z_0$) &
  $0.447^{\pm.002}$ &
  $0.633^{\pm.002}$ &
  $0.734^{\pm.002}$ &
  $0.513^{\pm.011}$ &
  $3.384^{\pm.008}$ &
  $9.181^{\pm.065}$ &
  $0.735^{\pm.055}$ 
   \\ 
MLD-1 ($\epsilon$) &
  $\boldsymbol{0.481}^{\pm.003}$ &
  $\boldsymbol{0.673}^{\pm.003}$ &
  $\boldsymbol{0.772}^{\pm.002}$ &
  $\boldsymbol{0.473}^{\pm.013}$ &
  $\boldsymbol{3.196}^{\pm.010}$ &
  $\boldsymbol{9.724}^{\pm.082}$ &
  $\boldsymbol{2.413}^{\pm.079}$ 
   \\   
\bottomrule
\end{tabular}%
}
% \vspace{-6pt}
\caption{Comparison of text-to-motion. ($cf.$ Tab. 1 for details.)}
\label{tab:tm:abl:humanml3d}
% \vspace{-12pt}
\end{table}

\section{Inference time}
\label{sec:appendix:inferencetime}
We provide a detailed ablation study with DDIM below.
In \cref{tab:tm:abl:scheduler}, 
MLD reduces the computational cost of diffusion models, which is the main reason for faster inference.
The iterations of diffusion further widen the gap in computational cost.
% %
Please note the bad FID of MDM with DDIM is mentioned in their GitHub issues \#76.
\begin{table}[h]
\centering
% \vspace{-6pt}
\resizebox{\columnwidth}{!}
{%
\begin{tabular}{@{}lrrrrrrrrlccccc@{}}
\toprule
\multirow{4}{*}{Methods} & \multicolumn{4}{c}{Total Inference Time (s) $\downarrow$} & \multicolumn{4}{c}{FLOPs (G) $\downarrow $} & \multirow{4}{*}{Parameter} & \multicolumn{4}{c}{FID $\downarrow $} \\
\cmidrule(lr){2-5} \cmidrule(lr){6-9} \cmidrule(lr){11-14}&\multicolumn{3}{c}{DDIM}& DDPM&\multicolumn{3}{c}{DDIM}& DDPM&&\multicolumn{3}{c}{DDIM}&DDPM\\
\cmidrule(lr){2-4} \cmidrule(lr){5-5} \cmidrule(lr){6-8} \cmidrule(lr){9-9} \cmidrule(lr){11-13} \cmidrule(lr){14-14}
& 50 & 100 & 200 & 1000& 50 & 100 & 200 & 1000&&50&100 & 200&1000\\

% & \multicolumn{3}{c}{DDIM} & DDPM  & 
% % \multirow{2.5}{*}{FLOPs}
% \multicolumn{2}{c}{FLOPs (G)}& Diffusion & \multicolumn{2}{c}{FID$\downarrow$} \\
% \cmidrule(lr){2-4}\cmidrule(lr){5-5}\cmidrule(lr){6-7}\cmidrule(lr){9-10} & 50 & 100 & 200 & 1000  &DDIM-50 & DDPM-1000 & Parameter & DDIM-50 & DDPM-1000  \\
 \toprule
 MDM
&225.28 & 456.70 & 911.36 & \textcolor{black}{4546.23}
% &1.657 &3.264 &6.654 & 24.74 
&597.97&1195.94&2391.89&11959.44&
$x \in \mathbb{R}^{196\times512}$
& 7.334&5.990&5.936&0.544\\ 

MLD
% &0.217&0.502&1.015&5.274 
&\textbf{10.24} & \textbf{16.38} & \textbf{28.67 }& \textbf{148.97}
&\textbf{29.86}&\textbf{33.12}&\textbf{39.61}&\textbf{91.60}& 
$z \in \mathbb{R}^{1\times256}$ 
&0.473&0.426&0.432&\textcolor{black}{0.568}\\ 
% \midrule
% \multirow{2}{*}{MLD-NoVAE} &FID$\downarrow$& & & & 0.544\\ 
% &AITS$\downarrow$&0.422&0.844&1.665& 8.799\\
% \midrule

\bottomrule
\end{tabular}%
}
% \vspace{-6pt}
\caption{Evaluation of inference time costs on text-to-motion: we evaluate the total inference time to generate 2048 motion clips with different diffusion schedules, floating point operations (FLOPs) counted by THOP library, the size of diffusion input, and FID.}
\label{tab:tm:abl:scheduler}
% \vspace{-10pt}
\end{table}

\section{Latent space visualization}
\label{sec:appendix:tsne}

We provide the visualizations of the t-SNE results on the latent space in  \cref{fig:tsne} to demonstrate how latent space evolves during the diffusion process with different actions.
From left to right, it shows the evolved latent codes during the inference of diffusion models.
\begin{figure}[htb]
    \centering
    % \vspace{-10pt}
    \includegraphics[width=1.0\linewidth]{rebuttal/TSNE.pdf}
    % \vspace{-18pt}
    \caption{Visualization of the t-SNE results on evolved latent codes $\hat{z}_t$ during the reverse diffusion process (inference) on action-to-motion task.
    $t$ is the diffusion step but ordered in the forward diffusion trajectory.
    $\hat{z}_{t=49}$ is the initial random noise. $\hat{z}_{t=0}$ is our prediction.
    We sample 30 motions for each action label.}
    \label{fig:tsne}
    % \vspace{-10pt}
\end{figure}

\section{Evaluation of Hyperparameters}
\label{sec:appendix:hyperparameters}

Here, we present two different experiments of text-to-motion on HumanML3D~\cite{Guo_2022_CVPR_humanml3d}. The first experiment is to change the dropout $p$ and scale in classifier-free diffusion guidance~\cite{ho2022classifier}. In \cref{tab:appendix:guidance}, we find that by changing dropout $p$ from $0.1$ to $0.25$, the text correspondences (R Precision) become worse but the motion quality (FID) gets better. It is the same as changing scale $s$ range from $7.5$ to $2.5$. Besides, some settings like $(0.25,7.5)$ achieve the best FID of 0.229, but we still suggest $(0.1,7.5)$ as dropout and scale $(p,s)$ for MLD models (\cref{experiments}) overall metrics.

Next, in \cref{tab:appendix:batchsize}, we experiment with batch sizes of 32, 64, 128, 256 and 512 under 8 Tesla V100 each with 32 GPU memory. We set it to 64 in our other experiments.
% refer to stable-diffusion E
% \subsection{Classifier-free Diffusion Guidance}
\label{appendix:guidance}
% uncondition factor

% F. Uncondition scale x
% MDiffuse_1107_VaeActor_transenc9_bs64_skip_lr1e4_clip_55_newvae6999
% MDiffuse_1102_VaeActor_transenc9_bs128_skip_lr1e4_clip_75_newvae6999

% \begin{table}[H]
% \centering
% \resizebox{0.75\columnwidth}{!}{%
% \begin{tabular}{@{}lcccccc@{}}
% \toprule
% \multirow{2}{*}{Models}  & Classifier-free & \multicolumn{1}{c}{R Precision} & \multicolumn{1}{c}{\multirow{2}{*}{FID$\downarrow$}} & \multirow{2}{*}{MM Dist.$\downarrow$} & \multirow{2}{*}{Diversity$\rightarrow$} & \multirow{2}{*}{MModality$\uparrow$} \\
%                           & Dropout & \multicolumn{1}{c}{Top 3$\uparrow$}       & \multicolumn{1}{c}{}                     &                          &                            &     \\ \toprule
% Real & - &
%   $0.797^{\pm.002}$ &
%   $0.002^{\pm.000}$ &
%   $2.974^{\pm.008}$ &
%   $9.503^{\pm.065}$ &
%   \multicolumn{1}{c}{-}
%   \\ \midrule
% MLD-1& $p=0.05$ & 
%   $0.766^{\pm.002}$	&$0.574^{\pm.013}$	&$3.237^{\pm.007}$&	$9.664^{\pm.069}$&	$2.433^{\pm.074}$ \\
% MLD-1 &$p=0.10$    & $0.772^{\pm.002}$ &	$0.473^{\pm.013}$ &	$3.196^{\pm.010}$ &	$9.724^{\pm.082}$ &	$2.413^{\pm.079}$\\
% MLD-1 &$p=0.15$ & $0.765^{\pm.002}$&	$0.311^{\pm.009}$&	$3.209^{\pm.007}$&	$9.649^{\pm.065}$&	$2.525^{\pm.070}$  \\
% MLD-1 &$p=0.20$ & 
% \\
% \bottomrule
% \end{tabular}%
% }
% % \vspace{2pt}
% \caption{Evaluation of classifer-free}
% \label{tab:ablation:klloss}
% \end{table}

\begin{table}[H]
\centering
\resizebox{0.8\columnwidth}{!}{%
\begin{tabular}{@{}lccccccc@{}}
\toprule
\multirow{2}{*}{Models}  & \multicolumn{2}{c}{Classifier-free} & \multicolumn{1}{c}{R Precision} & \multicolumn{1}{c}{\multirow{2}{*}{FID$\downarrow$}} & \multirow{2}{*}{MM Dist$\downarrow$} & \multirow{2}{*}{Diversity$\rightarrow$} & \multirow{2}{*}{MModality$\uparrow$} \\\cmidrule(l){2-3}
                          & Dropout & Scale & \multicolumn{1}{c}{Top 3$\uparrow$}       & \multicolumn{1}{c}{}                     &                          &                            &     \\ \toprule
Real & - &- &
  $0.797^{\pm.002}$ &
  $0.002^{\pm.000}$ &
  $2.974^{\pm.008}$ &
  $9.503^{\pm.065}$ &
  \multicolumn{1}{c}{-}
  \\ \midrule
MLD-1& $p=0.05$ &  $s=7.5$ &
  $0.766^{\pm.002}$	&$0.574^{\pm.013}$	&$3.237^{\pm.007}$&	$9.664^{\pm.069}$&	$2.433^{\pm.074}$ \\
MLD-1 &$p=0.10$  & $s=7.5$    & $\boldsymbol{0.772}^{\pm.002}$ &	$0.473^{\pm.013}$ &	$\boldsymbol{3.196}^{\pm.010}$ &	$9.724^{\pm.082}$ &	$2.413^{\pm.079}$\\
MLD-1 &$p=0.15$ & $s=7.5$ & $0.765^{\pm.002}$&	$0.311^{\pm.009}$&	$3.209^{\pm.007}$&	$9.649^{\pm.065}$&	$2.525^{\pm.070}$  \\
MLD-1 &$p=0.20$  & $s=7.5$ &$0.761^{\pm.002}$& $0.279^{\pm.011}$ &	$3.243^{\pm.009}$ &	$\boldsymbol{9.632}^{\pm.082}$ &	$2.651^{\pm.080}$\\
MLD-1 &$p=0.25$  & $s=7.5$ & $0.757^{\pm.002}$& $\boldsymbol{0.229}^{\pm.010}$&	$3.260^{\pm.008}$&	$9.649^{\pm.069}$&	$\boldsymbol{2.685}^{\pm.084}$\\
MLD-1 &$p=0.30$  & $s=7.5$ & $0.759^{\pm.002}$&	$0.289^{\pm.010}$&	$3.249^{\pm.008}$&	$9.670^{\pm.073}$&	$2.650^{\pm.082}$
\\
\midrule
MLD-1 &$p=0.10$  & $s=1.5$ &$0.648^{\pm.002}$&	$0.401^{\pm.019}$&	$3.857^{\pm.009}$&	$9.263^{\pm.056}$&$\boldsymbol{3.914}^{\pm.115}$\\
MLD-1 &$p=0.10$  & $s=2.5$ & $0.720^{\pm.002}$	&$\boldsymbol{0.350}^{\pm.013}$&	$3.441^{\pm.010}$	&$\boldsymbol{9.549}^{\pm.058}$&	$3.201^{\pm.098}$\\
MLD-1 &$p=0.10$  & $s=3.5$ &$0.745^{\pm.002}$&	$0.358^{\pm.011}$&	$3.299^{\pm.009}$&	$9.639^{\pm.065}$&	$2.890^{\pm.087}$\\
MLD-1 &$p=0.10$  & $s=4.5$ & $0.758^{\pm.002}$ &	$0.375^{\pm.011}$&	$3.232^{\pm.009}$&	$9.676^{\pm.069}$&	$2.701^{\pm.078}$ \\
MLD-1 &$p=0.10$  & $s=5.5$ & $0.764^{\pm.002} $	&$0.396^{\pm.011}$&	$3.202^{\pm.010}$&	$9.681^{\pm.072}$&	$2.577^{\pm.076}$  \\
MLD-1 &$p=0.10$  & $s=6.5$ & $0.767^{\pm.002}$ &$0.424^{\pm.011}$&	$\boldsymbol{3.191}^{\pm.009}$&	$9.658^{\pm.072}$& 	$2.498^{\pm.074}$  \\
MLD-1 &$p=0.10$  & $s=7.5$ & $\boldsymbol{0.772}^{\pm.002}$ &	$0.473^{\pm.013}$ &	$3.196^{\pm.010}$ &	$9.724^{\pm.082}$ &	$2.413^{\pm.079}$\\
MLD-1 &$p=0.10$  & $s=8.5$ & $0.768^{\pm.002}$ &	$0.504^{\pm.012}$ &	$3.207^{\pm.009}$ &	$9.604^{\pm.073}$ &	$2.413^{\pm.072}$  \\
MLD-1 &$p=0.10$  & $s=9.5$ & $0.766^{\pm.001}$&	$0.555^{\pm.012}$&	$3.227^{\pm.010}$&	$9.567^{\pm.072}$&	$2.394^{\pm.069}$ \\
\bottomrule
\end{tabular}%
}
\vspace{-6pt}
\caption{\textbf{Classifier-free Diffusion Guidance:} We study the influence of its hyperparameters, dropout $p$ and scale $s$ on text-to-motion.}
\label{tab:appendix:guidance}
\vspace{-6pt}
\end{table}

% fig factor = 3.5 4.5 5.5 6.5 7.5 8.5 9.5 10.5
% \begin{table}[H]
% \centering
% \resizebox{0.75\columnwidth}{!}{%
% \begin{tabular}{@{}lcccccc@{}}
% \toprule
% \multirow{2}{*}{Models}  & Classifier-free & \multicolumn{1}{c}{R Precision} & \multicolumn{1}{c}{\multirow{2}{*}{FID$\downarrow$}} & \multirow{2}{*}{MM Dist.$\downarrow$} & \multirow{2}{*}{Diversity$\rightarrow$} & \multirow{2}{*}{MModality$\uparrow$} \\
%                           & Scale & \multicolumn{1}{c}{Top 3$\uparrow$}       & \multicolumn{1}{c}{}                     &                          &                            &     \\ \toprule
% Real & - &
%   $0.797^{\pm.002}$ &
%   $0.002^{\pm.000}$ &
%   $2.974^{\pm.008}$ &
%   $9.503^{\pm.065}$ &
%   \multicolumn{1}{c}{-}
%   \\ \midrule
% MLD-1& $s=0.05$ & 
%   $0.766^{\pm.002}$	&$0.574^{\pm.013}$	&$3.237^{\pm.007}$&	$9.664^{\pm.069}$&	$2.433^{\pm.074}$ \\
% MLD-1 &$s=0.10$    & $0.772^{\pm.002}$ &	$0.473^{\pm.013}$ &	$3.196^{\pm.010}$ &	$9.724^{\pm.082}$ &	$2.413^{\pm.079}$\\
% MLD-1 &$s=0.15$ & $0.765^{\pm.002}$&	$0.311^{\pm.009}$&	$3.209^{\pm.007}$&	$9.649^{\pm.065}$&	$2.525^{\pm.070}$  \\
% MLD-1 &$s=0.20$ & 
% \\
% \bottomrule
% \end{tabular}%
% }
% % \vspace{2pt}
% \caption{Evaluation of text-based motion synthesis on HumanML3D~\cite{Guo_2022_CVPR_humanml3d}: we use metrics in \cref{tab:tm:comp:humanml3d} and provides real reference, the evaluation on with Autoencoder or VAE as our motion encoder and decoders.}
% \label{tab:ablation:klloss}
% \end{table}

% \subsection{Batch Size}

\begin{table}[H]
\centering
\vspace{-12pt}
\resizebox{0.75\columnwidth}{!}{%
\begin{tabular}{@{}lcccccc@{}}
\toprule
\multirow{2}{*}{Models}  & \multicolumn{1}{c}{\multirow{2}{*}{Batch Size}} & \multicolumn{1}{c}{R Precision} & \multicolumn{1}{c}{\multirow{2}{*}{FID$\downarrow$}} & \multirow{2}{*}{MM Dist$\downarrow$} & \multirow{2}{*}{Diversity$\rightarrow$} & \multirow{2}{*}{MModality$\uparrow$} \\
                          &  & \multicolumn{1}{c}{Top 3$\uparrow$}       & \multicolumn{1}{c}{}                     &                          &                            &     \\ \toprule
Real &-&
  $0.797^{\pm.002}$ &
  $0.002^{\pm.000}$ &
  $2.974^{\pm.008}$ &
  $9.503^{\pm.065}$ &
  \multicolumn{1}{c}{-}
  \\ \midrule
MLD-1 & 32 & $0.761^{\pm.003}$&	$0.445^{\pm.012}$&	$3.243^{\pm.010}$&	$9.751^{\pm.086}$&	$\boldsymbol{2.581}^{\pm.070}$
   \\
MLD-1 & 64  & $\boldsymbol{0.772}^{\pm.002}$ &	$0.473^{\pm.013}$ &	$\boldsymbol{3.196}^{\pm.010}$ &	$9.724^{\pm.082}$ &	$2.413^{\pm.079}$\\
MLD-1 & 128 & $0.771^{\pm.002}$&	$\boldsymbol{0.421}^{\pm.013}$&	$3.187^{\pm.008}$&	$\boldsymbol{9.691}^{\pm.080}$&	$2.370^{\pm.078}$ \\
MLD-1 & 256 & 
$0.770^{\pm.002}$&	$0.423^{\pm.010}$&	$3.211^{\pm.007}$&	$9.800^{\pm.070}$&	$2.401^{\pm.074}$
% $0.726^{\pm.002}$ &	$0.534^{\pm.016}$ &	$3.481^{\pm.011}$ &	$9.615^{\pm.081}$ &	$2.992^{\pm.117}$  
\\
MLD-1 & 512 & $0.769^{\pm.002}$ &	$0.446^{\pm.011}$&	$3.227^{\pm.010}$&	$9.772^{\pm.071}$&	$2.413^{\pm.072}$  \\

\bottomrule
\end{tabular}%
}
% \vspace{2pt}
\caption{\textbf{Batch Size:} We explore the evaluation of the batch size. We find the results are close and suggest 64 and 128 in this task.}
\label{tab:appendix:batchsize}
\end{table}

% fig factor = 3.5 4.5 5.5 6.5 7.5 8.5 9.5 10.5

\section{User Study}
\label{sec:appendix:userstudy}
For the pairwise comparisons of the user study presented in \cref{fig:appendix:user}, we use the force-choice paradigm to ask ``Which of the two motions is more realistic?'' and ``which of the two motions corresponds better to the text prompt?''. The provided motions are generated from 30 text descriptions, which are randomly generated from the test set of HumanML3D\cite{Guo_2022_CVPR_humanml3d} dataset. We invite 20 users and provide three comparisons, ours and MDM~\cite{mdm2022human}, ours and T2M~\cite{Guo_2022_CVPR_t2m}, ours and real motions from the dataset. 
Our MLD was preferred over the other state-of-the-art methods and even competitive to the ground troth motions.
\begin{figure}[h]
    \centering
    \includegraphics[width=0.9\linewidth]{figures/user_study.pdf}
    % \vspace{-10pt}
    \caption{\textbf{User Study:} Each bar indicates the preference rate of MLD over other methods. The red line indicates the 50\%. Please refer to the supplemental video for the comparisons of dynamic motion results.}
    \label{fig:appendix:user}
\end{figure}

\section{Motion Representations}
\label{sec:appendix:motionRepre}
Four relevant motion representations are summarized:

 \textbf{HumanML3D Format}~\cite{Guo_2022_CVPR_humanml3d} proposes a motion representation $x^{1:L}$ inspired by motion features in character control~\cite{starke2019neural, 2021-TOG-AMP, starke2022deepphase}. This redundant representation is quite suited to neural models, particularly variational autoencoders. Specifically, the $i$-th pose $x^i$ is defined by a tuple of root angular velocity $\dot{r}^a \in \mathbb{R}$ along Y-axis, root linear velocities $(\dot{r}^x, \dot{r}^z \in \mathbb{R})$ on XZ-plane, root height $r^y \in \mathbb{R}$, local joints positions $\mathbf{j}^p\in\mathbb{R}^{3N_j}$, velocities $\mathbf{j}^v\in\mathbb{R}^{3N_j}$ and rotations $\mathbf{j}^r\in\mathbb{R}^{6N_j}$ in root space, and binary foot-ground contact features $\mathbf{c}^f \in \mathbb{R}^4$ by thresholding the heel and toe joint velocities, where $N_j$ denotes the joint number, giving:
\begin{align}
 x^i = \{\dot{r}^a, \dot{r}^x, \dot{r}^z, r^y, \mathbf{j}^p, \mathbf{j}^v, \mathbf{j}^r, \mathbf{c}^f\}.
\end{align}
%
% However, \cite{Guo_2022_CVPR_humanml3d} clarifies that it is hard to convert back to SMPL parameters and proposes a 3D SMPL fitting process based on SMPLify\cite{bogo2016keep}.
%
% Our framework and MDM~\cite{mdm2022human} are reliable on this fitting to generate SMPL results.

\textbf{SMPL-based Format}~\cite{SMPL2015}. The most popular parametric human model, SMPL~\cite{SMPL2015} and its variants~\cite{MANO:SIGGRAPHASIA:2017, SMPLX2019} propose motion parameters $\theta$ and shape parameters $\beta$. $\theta \in \mathbb{R}^{3\times23+3}$ is rotation vectors for 23 joints and a root, and $\beta$ are the weights for linear blended shapes.
This representation is popular in markerless motion capture~\cite{he2021challencap,chen2021sportscap,VIBE_CVPR2020}.
By involving the global translation $r$, the representation is formulated as:
\begin{align}
 x^i = \{r, \theta, \beta\}.
\end{align}

% 夸smpl表彰人体
% 公式表达动作 参考下面的公式

\textbf{MMM Format}~\cite{terlemez2014master}. Master Motor Map (MMM) representations propose joints angle parameters by adopting a uniform skeleton structure with 50 DoFs. And most recent methods ~\cite{ahuja2019language2pose,ghosh2021synthesis,petrovich22temos} on text-to-motion task followed preprocess procedure in ~\cite{holden2016deep} which transform joint rotation angles to $J=21$ joints XYZ coordinates, giving $p_m\in \mathbb{R}^{3J}$,  and global trajectory $t_{root}$ for the root joint. 
The preprocessed representation can be formulated as 
\begin{align}
 x^i = \{p_m, t_{root}\}.
\end{align}

% xxx 特殊的骨架格式

\textbf{Latent Format}~\cite{SMPL2015}. 
% 讲 大家广泛使用 vae 以及latent
% 也可以有效的表彰 动作
% 我们也把latent当做是motion representation的一种
Latent representations are widely used in neural models~\cite{petrovich21actor, petrovich22temos,guo2020action2motion, chen2022learning}.
We recognize it as motion representation in latent space.
By leveraging VAE models, latent vectors can represent plausible motions as:
\begin{align}
 \hat{x}^{1:L} = \mathcal{D}(z), z = \mathcal{E}(x^{1:L})
\end{align}

\section{Details on Motion Latent Diffusion Models}
\label{appedix:method:detail}
% Methods details
\subsection{Details Information on Variational Autoencoder Models}
\label{sec:appendix:loss}
%We train Variational Autoencoder Models $\mathcal{V}$ on .
\jb{We take HumanML3D~\cite{Guo_2022_CVPR_humanml3d} and its motion representation (\cref{sec:appendix:motionRepre}) as an example here to explain our loss details of Variational Autoencoder Models $\mathcal{V}$.}
%
% The models is optimized with two loss terms.
%
The motion $x^{1:L}$ includes joint features and is supervised with data term by mean squared error:
\begin{align}
% (x^{1:L}, \mathcal{D}(\mathcal{E}(x^{1:L})))
\mathcal{L}_{data} = \left\| x^{1:L} - \mathcal{D}(\mathcal{E}(x^{1:L})) \right\|^2.
\end{align}
To regularize latent space as a standard variational autoencoder~\cite{kingma2013auto}, we employ a Kullback-Leibler term between $q(z|x^{1:L}) = \mathcal{N}\left(z ; \mathcal{E}_\mu, \mathcal{E}_{\sigma^2}\right)$ and a standard Gaussion distribution $\mathcal{N}\left(z;0,1\right)$.
The full training loss of the VAE model $\mathcal{V}$ follows:
\begin{align}
\mathcal{L}_{\mathcal{V}} = \mathcal{L}_{data}(x^{1:L}, \mathcal{D}(\mathcal{E}(x^{1:L}))) + \lambda_{reg}\mathcal{L}_{reg}(x^{1:L};\mathcal{E},\mathcal{D}),
\end{align}
where $\lambda_{reg}$ is a low weight to control the regularization. 
The KIT~\cite{Plappert2016kit}, HumanAct12~\cite{guo2020action2motion} and UESTC~\cite{ji2018large} dataset processed by \cite{petrovich22temos,petrovich21actor} also supports SMPL-based~\cite{SMPL2015} motion representation.
Here we list the loss terms for this representation.
The data term formulates as followed:
\begin{align}
    \label{eq:vae:humanml}
    \mathcal{L}_{data} = \sum_{i=1}^L \left\|{r}^i  -\hat{{r}}^i \right\|_2 + \sum_{i=1}^L \left\|{\theta}^i  -\hat{{\theta}}^i \right\|_2 +  \left\|{\beta}  -\hat{{\beta}} \right\|_2.
\end{align}
Here the motion is $x^{1:L} = \{{r}^i, {\theta}^i, {\beta}\}^{L}_{i=1}$, which includes global translation ${r}^i$, pose parameter ${\theta}^i$ and shape parameter ${\beta}$ of the $i$-th frame. 
To enhance the full-body supervision, the reconstruction term on the SMPL vertices follows:
\begin{align}
    \mathcal{L}_{\mathrm{mesh}} = \sum_{i=1}^L \left\| {V}_i - M(\hat{{r}}^i, \hat{{\theta}}^i,\hat{{\beta}}^i) \right\|^2,
\end{align}
where the body reconstruction function $M(\cdot)$ is from the differentiable SMPL layer, while the vertices ${V}_i$ are calculated with the ground truth motion parameters using the same layer.
The reconstruction loss builds global supervision on almost all predicted parameters $ \{{r}_t, {\theta}_t, {\beta}\} $ and shows a reliable supervision~\cite{petrovich21actor} for motion generation.
The full objective on SMPL-based motion representation reads:
\begin{align}
    \label{eq:vae:smpl}
    \mathcal{L}_{\mathcal{V}} = \mathcal{L}_{data} + \lambda_{mesh}\mathcal{L}_{mesh} + \lambda_{reg}\mathcal{L}_{reg}.
\end{align}
% 总体解释，每个loss的目的和作用
where $\lambda_{mesh}$ is the weight to enhance the supervision on the full-body vertices. Besides, the regularization term is the same as the Kullback-Leibler term in \cref{eq:vae:humanml}.
In practice, the shape parameters, as part of global motion features, increase the complexity of motion generation and influence joint positions. 
% Thus, the shape error causes the foot sliding easily. 
% \cref{sec:appendix:motionRepre}, we 
We finally utilize the objective of ~\cref{eq:vae:humanml} to train our text-based models and \cref{eq:vae:smpl} to train action-based models in comparisons and evaluations.

\subsection{Network Architectures}
The details of network architecture are shown as \cref{fig:appendix:net}, our MLD comprises three main components, motion encoder $\mathcal{E}$, motion decoder $\mathcal{D}$ and latent denoiser $\epsilon_\theta$. Please refer to the following figure and \cref{tab:appendix:details} for more details.
% 2.1 network structure
% 2.3 implement details

\begin{figure}[h]
    \centering
    \includegraphics[width=0.85\linewidth]{figures/network.pdf}
    \caption{Network architecture of our conditional MLD. We explain each component in its right bottom part and the loss terms in \cref{sec:appendix:loss}.  }
    \label{fig:appendix:net}
\end{figure}

% \newpage
\subsection{Implementation Details}
For the experiments on text-to-motion, action-to-motion, and unconditional motion synthesis, we implement MLDs with various latent shapes as follows. Specifically, MLD-7 works best in evaluating VAE models (\cref{tab:mr:ablation}), and MLD-1 wins these generation tasks (\cref{tab:tm:comp:humanml3d,,tab:tm:comp:kit,,tab:comp:action,,tab:ablation:uncon}). In other words, MLD-7 wins the first training stage for the VAE part, while MLD-1 wins the second for the diffusion part. We thought MLD-7 should perform better than MLD-1 in several tasks, but the results differ. The main reason for this downgrade of a larger latent size, we believe, is the small amount of training data. HumanML3D only includes 15k motion sequences, much smaller than billions of images in image generation. MLD-7 could work better when the motion data amount reaches the million level.
% \textbf{Sampling Details for Unconditional Generation.} Motion Latent Diffusion (MLD) models support two types of unconditional samplings, sampling from latent distribution and sampling before the denoising steps of diffusion models.
% %
% We employ the same standard Gaussian distribution $\mathcal{N}(z;0,1)$ for two samplings.
% %
% These generated latent vectors rely on the decoder $\mathcal{D}$ for motion reconstructions.
% quite similar

\begin{table}[H]
\centering
\resizebox{0.7\columnwidth}{!}{%
\begin{tabular}{@{}lccccc@{}}
\toprule
\multirow{2}{*}{} &  MLD-1 & MLD-2 & MLD-5 & MLD-7 & MLD-10
 \\ \toprule
$z$-shape & $1\times 256$& $2\times 256$& $5\times 256$& $7\times 256$& $10\times 256$
\\
% $|Z|$ &
% \\
Training Diffusion steps & 1000 &1000 &1000 &1000 & 1000 
\\
Inference Diffusion steps  & 50 &50 &50 &50 & 50 
\\
Noise Schedule & scaled linear & scaled linear & scaled linear & scaled linear & scaled linear
\\
Denoiser Heads Number & 4 & 4& 4& 4& 4
\\
Denoiser Transformer Layers & 9 &9 & 9 & 9 & 9 
\\
Conditioning & concat& concat& concat& concat& concat
\\
\midrule
Embedding Dimension & 256 & 256 & 256 & 256 & 256
\\
VAE Heads Number  & 4 & 4& 4& 4& 4
\\
VAE Transformer Layers & 9 & 9 & 9 & 9 & 9 
\\\midrule
Model Size (w/o clip) & 26.9M&26.9M&26.9M&26.9M&26.9M
\\
Diffusino Batch Size & 64 &64 &64 &64 &64
\\
Diffusion Epochs & 2000& 2200& 2400& 2600& 2800
\\
VAE Batch Size & 128 &128 &128 &128 &128
\\
VAE Epochs & 4000& 4500& 5000& 5500& 6000
\\
Learning Rate & 1e-4& 1e-4& 1e-4& 1e-4& 1e-4
\\
\bottomrule
\end{tabular}%
}
% \vspace{2pt}
\caption{Hyperparameters for the conditional MLDs in experiments. We train these models on 8 Tesla V100. The smaller latent shape lowers the computational requirements and provides faster inference. }
\label{tab:appendix:details}
\end{table}

\section{Metric Definitions}
\label{appedix:metrics:details}
% AITS 详细计算流程

% motion quality, generation diversity, condition matching, and time costs.
We provide more details of evaluation metrics in \cref{sec:comp:metric} as follows.

% \cx{xx R-Percision xx  Multimod. xxx MM Dist xxKID xx}
\textbf{Motion Quality}. \jb{
Frechet Inception Distance (FID) is our principal metric to evaluate the distribution similarity between generated and real motions, calculated with the suitable feature extractor~\cite{guo2020action2motion,petrovich21actor,Guo_2022_CVPR_t2m} for each dataset. 
% and use Kernel Inception Distance (KID) \cite{binkowski2018demystifying} as an supplement following \cite{raab2022modi}.
}
Besides, to evaluate the motion reconstruction error of VAEs, we use popular metrics in motion capture~\cite{VIBE_CVPR2020, chen2021sportscap, vonMarcard2018}, 
MPJPE, and PAMPJPE~\cite{gower1975generalized} for global and local errors in millimeter, 
% Mean Per Joint Position Error (MPJPE) and Procrustes Aligned MPJPE (PAMPJPE)~\cite{gower1975generalized} for global/local errors in millimeter, 
Acceleration Error (ACCL) for the quality on temporal.

\textbf{Generation Diversity}. \jb{Following ~\cite{guo2020action2motion,chuan2022tm2t}, we use Diversity (DIV) and MultiModality (MM) to measure the motion variance across the whole set and the generated motion diversity within each text input separately. Here we take the text-to-motion task as an example to explain the calculation steps and for other tasks the operations are similar. To evaluate Diversity, all generated motions are randomly sampled to two subsets of the same size $X_d$ with motion feature vectors $\{x_1,..,x_{X_d}\}$ and $\{x^{'}_1,..,x^{'}_{X_d}\}$ respectively. Then diversity is formalized as:
\begin{equation*}
    \text{DIV} = \frac{1}{X_d} \sum_{i=1}^{X_d} || x_i - x^{'}_{i} ||.
\end{equation*}
To evaluate MultiModality, a set of text descriptions with size $J_m$ is randomly sampled from all descriptions. Then two subsets of the same size $X_m$ are randomly sampled from all motions generated by $j\text{-th}$ text descriptions, with motion feature vectors $\{x_{j,1},..,x_{j,X_m}\}$ and $\{x^{'}_{j,1},..,x^{'}_{j,X_m}\}$ respectively. The multimodality is calculated as:

\begin{equation*}
    \text{MM} = \frac{1}{J_m \times X_m} \sum_{j=1}^{J_m} \sum_{i=1}^{X_m}|| x_{j,i}- x^{'}_{j, i} ||.
\end{equation*}

}

\textbf{Condition Matching}.
\jb{For the text-to-motion task, \cite{Guo_2022_CVPR_t2m} provides motion/text feature extractors to produce geometrically closed features for matched text-motion pairs, and vice versa. Under this feature space, 
motion-retrieval precision (R Precision) first mix generated motion with 31 mismatched motions and then calculates the text-motion top-1/2/3 matching accuracy, and Multi-modal Distance (MM Dist) that calculates the distance between generated motions and text.
For action-to-motion, for each dataset \cx{a pretrained recognition model~\cite{guo2020action2motion,petrovich21actor}} is used to calculate the average motion Accuracy (ACC) for action categories.
}

% MM Dist
% R-Percision
% Accuracy
\textbf{Time Costs}. To evaluate the computing efficiency of diffusion models, especially the inference efficiency, we propose Average Inference Time per Sentence (AITS) measured in seconds. In our case, we calculate AITS ($cf.$ \cref{fig:comp:time}) on the test set of HumanML3D~\cite{Guo_2022_CVPR_humanml3d}, set the batch size to one, and ignore the time cost for model and dataset loading parts.
